# Supplementary material for: SkillEvolBench: Benchmarking the Evolution from Episodic Experience to Procedural Skills
Source: arXiv:2605.24117 source file (2026-05-22)
Supplement: Supplementary file 1 [file Tier3.tex]

% \subsection{Exploring Whether Larger Skill Libraries Improve Frozen Evaluation}

% This ablation asks whether agents can extract enough reusable information from
% their execution traces to enrich the skill library beyond a single
% \texttt{SKILL.md} instruction file. The trace contains concrete evidence:
% commands that were repeatedly re-derived, validation scripts the agent wished
% it had, schema details discovered at runtime, lookup tables, examples, and
% templates. A capable Skill Author should be able to turn such evidence into
% persistent resources under \texttt{scripts/}, \texttt{references/}, and
% \texttt{assets/}. The central question is therefore not simply whether larger
% libraries are better. It is whether trace evidence contains enough reusable
% structure for the authoring model to extract, package, and attach it to the
% right procedural trigger.

% We use Tier-3 forcing as a diagnostic for this question. If the author can
% extract useful information from traces, then \textsc{Always+Tier3} should both
% produce richer libraries and preserve or improve frozen deployment success. If
% the author only produces additional files without reliable procedural value,
% then the library will grow while ESR remains flat or drops. The analysis below
% therefore separates two outcomes: \emph{enrichment capacity}, measured by the
% number of persisted skill resources, and \emph{useful enrichment}, measured by
% whether those resources improve ESR.
% \subsubsection{Tier-3 Resource Bundling Prompt}
% \label{app:tier3_prompt_comparison}

% Skills are intended to be reusable procedural
% memory rather than short textual hints. Intuitively, a richer skill should be
% more useful: executable helpers can remove brittle repeated commands,
% reference files can preserve long tables or API notes without bloating
% \texttt{SKILL.md}, and assets can provide reusable templates or schemas.
% The Tier-3 setting tests this intuition directly. It keeps the surrounding
% Skill Author interface fixed, but changes the revision instruction so that
% resource bundling is mandatory rather than optional.

% Importantly, the non-Tier-3 condition is not a ban on auxiliary files. The
% default \texttt{free\_form} strategy allows the Skill Author to add
% \texttt{scripts/}, \texttt{references/}, or \texttt{assets/} when they
% materially help. By contrast, the \texttt{tier3\_required} strategy forces
% each eligible revision to include at least one such resource under an existing
% skill. This creates a controlled comparison between ordinary free-form skill
% editing and an aggressive resource-bundling policy.

% \newtcblisting{skillpromptbox}[2][]{
%   enhanced,
%   breakable,
%   listing only,
%   colback=gray!3,
%   colframe=black!50,
%   coltitle=white,
%   colbacktitle=black!72,
%   title={#2},
%   fonttitle=\bfseries\small,
%   boxed title style={
%     sharp corners,
%     boxrule=0pt,
%   },
%   arc=1mm,
%   boxrule=0.45pt,
%   left=1.4mm,
%   right=1.4mm,
%   top=1.0mm,
%   bottom=1.0mm,
%   listing options={
%     basicstyle=\ttfamily\footnotesize,
%     breaklines=true,
%     columns=fullflexible,
%     keepspaces=true,
%     showstringspaces=false,
%     upquote=true
%   },
%   #1
% }

% \begin{skillpromptbox}{Shared structured edit interface}
% Return EXACTLY one JSON object with these keys:

% {
%   "summary": "<one short sentence describing the change>",
%   "operation_type": "revise" | "narrow" | "replace" | "create",
%   "upsert_files": {
%     "<slug>/SKILL.md": "<full new SKILL.md content>",
%     "<slug>/scripts/<file>": "<optional, only if SKILL.md cites it>",
%     "<slug>/references/<file>": "<optional, only if SKILL.md cites it>",
%     "<slug>/assets/<file>": "<optional, only if SKILL.md cites it>"
%   }
% }

% Always include FULL file content -- never diffs. Include only files you
% actually edited or created. No commentary outside the JSON.
% \end{skillpromptbox}

% \begin{skillpromptbox}{Without forced Tier-3: free-form revision mode}
% Make whatever edit best closes the gap exposed by the failure.
% Edit SKILL.md and -- when it materially helps -- add executable
% `scripts/`, on-demand `references/`, or `assets/` files.
% Cite every Tier-3 file you add from the SKILL.md body with a
% clear "when to read / run" trigger; uncited files will be rejected.
% Do NOT inflate the body for its own sake; size the change to the gap.
% \end{skillpromptbox}

% \begin{skillpromptbox}{With forced Tier-3: tier3-required revision mode}
% MANDATORY for this revision: upsert_files MUST include at least ONE new
% or updated file under `<slug>/scripts/`, `<slug>/references/`, or
% `<slug>/assets/`. A SKILL.md-only patch will be REJECTED by the parser.

% For folder choice + naming + hard rules, follow system spec section 6.
% The summary below is just a decision guide for picking the folder;
% spec 6 is the binding contract for HOW to write the file.

% DECISION GUIDE for this trial:
%   - Trace shows the agent re-deriving fragile multi-step logic, OR running
%     the same ad-hoc command repeatedly
%       -> bundle as `<slug>/scripts/<verb_object>.py`
%          and cite the exact command from SKILL.md.
%   - Trace shows the agent looking up long enum / API error table / vendored
%     doc that would bloat SKILL.md
%       -> move to `<slug>/references/<topic>.md` and cite the trigger
%          ("read this if X happens") in SKILL.md.
%   - Trace shows the agent reproducing a fixed output structure
%     (template / schema / config skeleton)
%       -> bundle as `<slug>/assets/<name>.<ext>` and tell SKILL.md to copy/fill.

% If a suitable Tier-3 file already exists in the target skill, UPDATE it in
% place -- do NOT create a near-duplicate.

% ADDITIVE BIAS still applies: cite this Tier-3 file from SKILL.md with a clear
% "when to run / read / copy" trigger. Uncited files are dead weight and rejected.
% \end{skillpromptbox}

% The parser enforces the distinction above. In \texttt{tier3\_required} mode,
% \texttt{upsert\_files} must contain at least one Tier-3 path under an existing
% target skill. A \texttt{SKILL.md}-only revision is invalid for this setting.
% Thus, the comparison asks whether forcing richer skill artifacts improves
% reuse beyond ordinary free-form skill revision, while keeping the trajectory
% evidence, verifier feedback, and Skill Author call surface unchanged.

% \subsubsection{Results and Library Size}
% \input{Figure_tex/library-size-esr}
% \label{app:tier3_results_library_size}

% \input{Table_tex/No-skill vs tier 3}
% The results separate artifact extraction from functional enrichment. Forced
% Tier-3 authoring does make agents write richer libraries: the
% \textsc{Always+Tier3} variants generally add more files under
% \texttt{scripts/}, \texttt{references/}, and \texttt{assets/}. This indicates
% that agents can identify trace-derived material that appears reusable. However,
% \Cref{tab:noskill_vs_always_tier3_compact} and
% \Cref{fig:library_size_vs_esr_model_specific} show that this extraction step is
% not enough to guarantee better frozen deployment. Many points in
% \Cref{fig:library_size_vs_esr_model_specific} move rightward without moving
% upward: the library grows, but ESR stays flat or decreases.

% The positive cases show that trace enrichment can be useful when the added
% resources capture stable procedures that the task-solving agent can actually
% reuse. \textsc{Claude Opus 4.6} improves under
% \textsc{SelfGen-Always+Tier3}, from \(37.8\%\) to \(40.0\%\) ESR, and
% \textsc{Gemini 3.1 Pro} improves under \textsc{Curated-Always+Tier3}, from
% \(35.6\%\) to \(40.0\%\). These results suggest that some traces do contain
% procedural details that are not fully preserved in the compact
% \texttt{SKILL.md} body alone. In those cases, Tier-3 files can serve their
% intended role: preserving reusable validation routines, reference material,
% templates, or executable helpers that future agents can load on demand.

% The failure cases show where current trace enrichment breaks down.
% \textsc{GPT-5.4} reaches its highest ESR with \textsc{Curated-Always}, while
% the larger \textsc{Curated-Always+Tier3} and
% \textsc{SelfGen-Always+Tier3} libraries reduce ESR. \textsc{Gemini 3 Flash}
% is the clearest overload case: its \textsc{SelfGen-Always+Tier3} library is
% among the largest, but ESR drops from \(35.6\%\) under \textsc{No-Skill} to
% \(27.8\%\). \textsc{Claude Sonnet 4.5} also drops from \(35.6\%\) to
% \(30.0\%\) under \textsc{SelfGen-Always+Tier3}. These drops suggest that
% forced enrichment can preserve trace details that look useful locally but do
% not transfer. Added resources may encode episode-specific assumptions,
% over-specific validators, stale context, or weakly triggered files that
% increase retrieval burden during frozen evaluation.

% Thus, the answer to the trace-enrichment question is only partially positive.
% Agents can extract more information from traces and package it as persistent
% skill resources, but they do not yet reliably extract the \emph{right}
% information. The limiting factor is selective enrichment: deciding which trace
% details are stable enough to persist, how to organize them as procedural
% resources, and when a future agent should load them. Tier-3 therefore exposes
% the same abstraction bottleneck from another angle. More capacity helps only
% when it is controlled; otherwise, richer libraries become procedural clutter
% rather than more reliable skills.
